# Supplementary material for: Quantum emission assisted by energy landscape modification in pentacene-decorated carbon nanotubes
Source: arXiv:2103.10665 ancillary file (2021-03-19)
Supplement: Supplementary file 1 [file PentaceneDecoration_SI.pdf]

# Supplementary Information

## Quantum emission assisted by energy landscape modification in pentacene-decorated carbon nanotubes

Zhen Li[1, 2], Keigo Otsuka[2], Daiki Yamashita[1], Daichi Kozawa[1], Yuichiro K. Kato[1, 2]

*[1]Quantum Optoelectronics Research Team, RIKEN Center for Advanced Photonics, Saitama 351-0198, Japan*

*[2]Nanoscale Quantum Photonics Laboratory, RIKEN Cluster for Pioneering Research, Saitama 351-0198, Japan*

1. Transmission electron microscope (TEM) images of pentacene-decorated CNTs

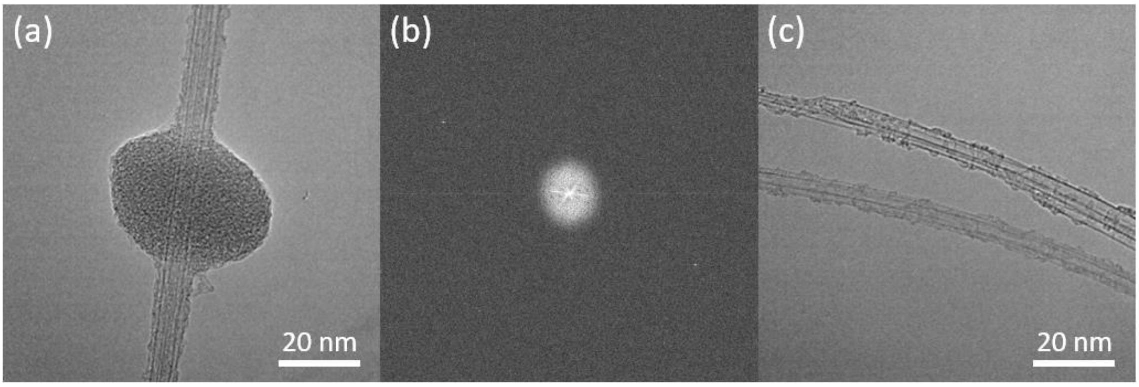


FIG. S1. (a) TEM image of a decorated pentacene particle. (b) Fast-Fourier transform of the TEM image in (a). (c) TEM image of the undecorated regions of CNTs. TEM characterization is performed using a JEOL JEM-2100F/SP operated at 200 kV.

2. Surface profiler scans of pentacene films on the sample substrate

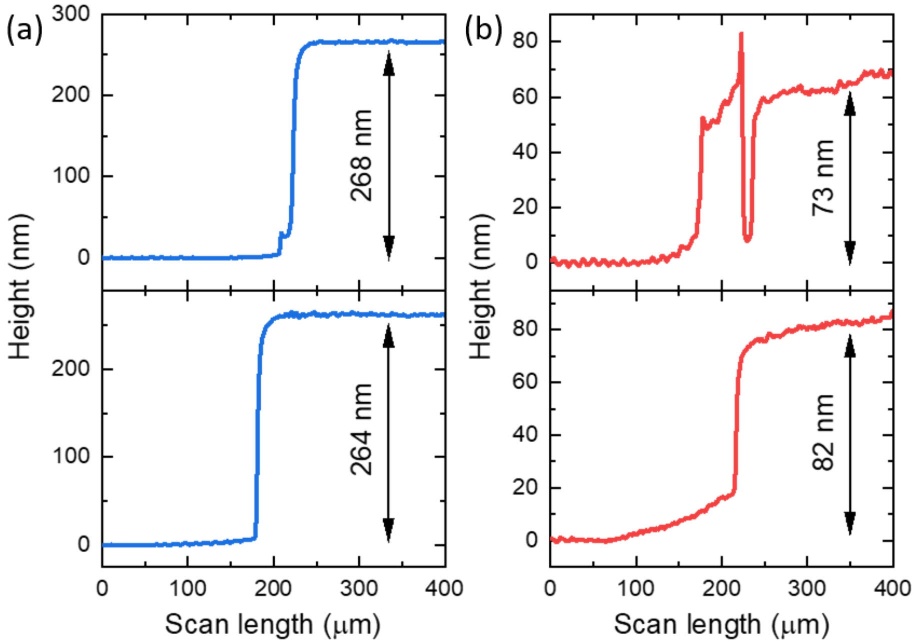


FIG. S2. Surface profiler scans taken at different locations of the sample substrates deposited with pentacene films having a nominal thickness of (a) 100 nm and (b) 50 nm, respectively.

## 3. Method to obtain the percentage of CNTs decorated with pentacene particles

After air-suspended CNTs are synthesized on a trenched substrate, automated PL trench scans are performed throughout the trenches to locate bright CNTs. The coordinates of the bright CNTs are then recorded, and automated polarization-dependent PL, PLE spectroscopy and PL imaging are carried out on the CNTs individually. After pentacene decoration, the same CNTs are characterized again by the automated measurements. The polarization-dependent PL intensity plots before and after pentacene decoration are compared in order to verify that the same CNT has been measured. To obtain the percentage of pentacene-decorated CNTs, above procedure is applied to two samples deposited with 4 and 9 nm pentacene film, respectively. The total number of individually suspended CNTs in these samples is about 400. Since the presence of a pentacene particle on the CNT will give rise to an extra peak in the PLE map as shown in Fig. 2(c), the percentage of CNTs decorated with pentacene particles can be obtained by counting the number of CNTs whose PLE map shows an extra peak.

## 4. Definition of the "pristine CNT" considering the effect of water molecules in air

Before pentacene decoration, detailed PL measurements of individual CNTs are carried out after automated PL trench scans that typically finish at least 10 hours after the CNTs are synthesized. During the 10-hour period, water molecules in air can adsorb onto the CNTs. Immediately before the detailed PL measurements, the amount of water molecules adsorbed onto such CNTs and the spectral redshifts induced by molecular adsorption are considered to have reached saturation [1-3]. In this work, we define the pristine CNTs as the CNTs adsorbed with sufficient amount of water molecules from air.

5. Typical PL spectra with and without the bandpass filter

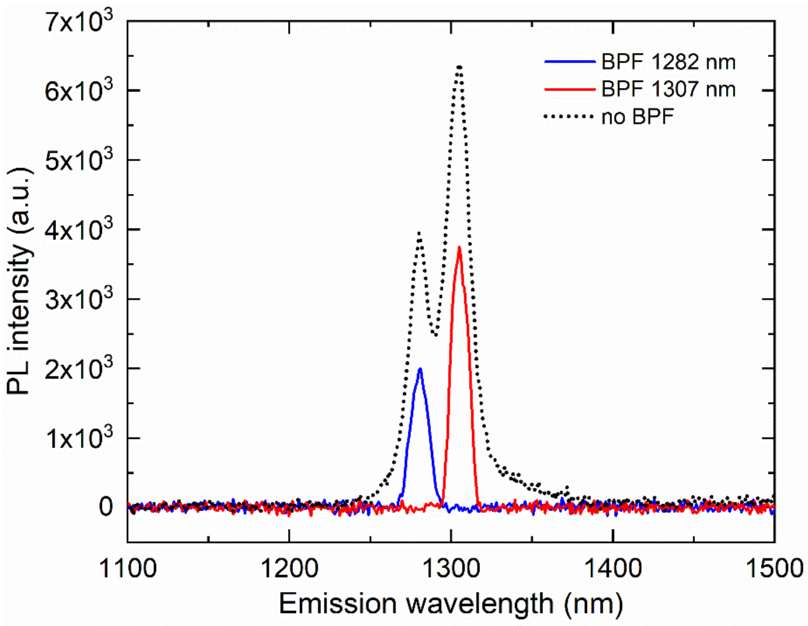


FIG. S3. Typical PL spectrum of a pentacene-decorated CNT without using the bandpass filter (black dots). PL spectra of the undecorated peak (blue curve) and the decorated peak (red curve) from the same CNT when using a rotatable bandpass filter with a standard central wavelength of 1350 nm and full width at half maximum of 12 nm. The central wavelength of the bandpass filter is tuned to the actual emission wavelength of each peak by changing its angle with respect to the incident light. The CW laser is kept at an excitation wavelength of 780 nm and $P$ =10 μW.

6. Decay and $g^{(2)}(0)$ data from more CNTs

| CNT # | Peak assignment | $E_{11}$ (eV) | $E_{22}$ (eV) | $g^{(2)}(0)$ | $\tau_1$ (ps) | $\tau_2$ (ps) |
|---|---|---|---|---|---|---|
| 1 | Undecorated | 0.957 | 1.588 | 0.44 | 81.6 | 724.5 |
| | Decorated | 0.940 | 1.584 | 0.48 | 81.8 | 704.3 |
| 2 | Undecorated | 0.958 | 1.587 | 0.68 | 75.1 | 531.5 |
| | Decorated | 0.945 | 1.580 | 0.50 | 84.1 | 439.9 |
| 3 | Undecorated | 0.967 | 1.585 | 0.49 | 86.2 | 689.7 |
| | Decorated | 0.955 | 1.583 | 0.38 | 81.0 | 684.2 |
| 4 | Undecorated | 0.950 | 1.578 | 0.60 | 59.6 | 236.0 |
| | Decorated | 0.939 | 1.575 | 0.71 | 61.7 | 222.6 |
| 5 | Undecorated | 0.955 | 1.577 | 0.71 | 57.3 | 159.5 |
| | Decorated | 0.942 | 1.572 | 0.58 | 53.1 | 178.6 |
| 6 | Undecorated | 0.956 | 1.585 | 0.68 | 59.3 | 536.3 |
| | Decorated | 0.945 | 1.581 | 0.61 | 62.4 | 835.4 |
| 7 | Undecorated | 0.947 | 1.584 | 0.64 | 55.2 | 548.8 |
| | Decorated | 0.937 | 1.583 | 0.61 | 69.6 | 846.0 |
| 8 | Undecorated | 0.956 | 1.587 | 0.60 | 75.5 | 522.7 |
| | Decorated | 0.941 | 1.584 | 0.44 | 79.2 | 486.2 |

Table S1. Decay and $g^{(2)}(0)$ data for the undecorated and decorated peak from eight (9,7) CNTs decorated with pentacene particles. The decay curves are fit by a biexponential function convoluted with the IRF. Pulsed laser is tuned to the excitation energy $E_{22}$ with $P = 20$ nW.

References


[1] Ishii, A.; Yoshida, M.; Kato, Y. K. Exciton diffusion, end quenching, and exciton-exciton annihilation in individual air-suspended carbon nanotubes. Phys. Rev. B **91**, 125427 (2015).

[2] Uda, T.; Tanaka, S.; Kato, Y. K. Molecular screening effects on exciton-carrier interactions in suspended carbon nanotubes. Appl. Phys. Lett. **113**, 121105 (2018).

[3] Ishii, A.; Machiya, H.; Kato, Y. High Efficiency Dark-to-Bright Exciton Conversion in Carbon Nanotubes. Phys. Rev. X **9**, 041048 (2019).
